# Supplementary material for: Beating Adversarial Low-Rank MDPs with Unknown Transition and Bandit Feedback
Source: arXiv:2411.06739 source file (2024-11-11)
Supplement: Supplementary file 1 [file appendix-full-infomation.tex]

\section{Proof of \cref{thm:full-info} (Model-Based, Full Information)}\label{app: model based full info}

Our confidence set construction is the same as that of \cite{uehara2021pessimistic} and we also adopt their analysis shown in \cref{lem:confidence set} following standard MLE analysis.

\begin{lemma}[Page 28-29 in \cite{uehara2021pessimistic}] \label{lem:confidence set} For any $t \in [T]$ and $h \in [H]$, with probability $1 - \frac{1}{T^2}$, let $\{\pi^i\}_{i=1}^T$ be the policies played in \cref{alg:full-info} and $\{\cP_h^t\}_{t=1}^H$ is the confidence set define in \cref{line:confidence} of \cref{alg:full-info}, we have $P_h^\star \in \cP_h^t$ and
\begin{align*}
 \sum_{i=1}^{t} \E^{\pi^i}\left[\left\|P_h(\cdot \mid  \x_h, \a_h) - P_h^\star(\cdot \mid  \x_h, \a_h)\right\|_1^2\right] \le c\log\left(|\Phi||\Upsilon| T\right), \,\, \forall P_h \in  \cP_h^t,
\end{align*}    
where $c$ is a universal constant. 
\end{lemma}

Let $\cE$ be the success event of \cref{lem:confidence set} holds for all $t \in [T]$ and $h \in [H]$. Applying the union bound,  $\cE$ happens with probability $1 - \frac{H}{T}$. Since $\mathrm{Reg}_T(\pi) \le HT$, for all $\pi\in \Pi$, we have $\E\left[\mathrm{Reg}_T(\pi)\cdot \indi\left\{\cE^c\right\}\right] \le H^2$. Thus, in the following analysis, we only consider the regret under the event $\cE$.

Our following proof is based on the dilated bonus lemma \cref{lem:dilated bonus} proposed by \cite{luo2021policy}. 

\begin{lemma}[Lemma B.1 in \cite{luo2021policy}] 
Suppose that for some non-nagative bonus functions $\tb_h^t$, a sequence of transition $\tp_{1:H}^t$, policy $\pi^t$, and scalar $v>0$,  we have for all $t \in [T]$, all $(x,a)\in \cX \times \cA$ for all $h \in [H]$, 
\begin{align}
\tB_h^t(x,a) &:= \tb_h^t(x,a) + \left(1 + \frac{1}{H}\right)\cdot \E_{\x_{h+1} \sim \tp_h^t(\cdot|x,a)}\E_{\a_{h+1} \sim \pi^t_{h+1}(\cdot \mid \x_{h+1})}\left[\tB_{h+1}^t(\x_{h+1}, \a_{h+1})\right] \nonumber
\\&\ge \tb_h^t(x,a) + \left(1 + \frac{1}{H}\right)\cdot\E^{\pi^t}\left[\tB_{h+1}^t(\x_{h+1}, \a_{h+1})\mid\x_h=x,\a_h=a \right], 
\label{eqn:B condition}
\end{align}
and for any policy $\pi^\star$, suppose that our algorithm guarantees
\begin{align}
&\E^{\pistar}\left[\sum_{t=1}^T\sum_{h=1}^H\left\langle Q_{h}^{\pi^t}(\x_h,\cdot) - \tB_h^t(\x_h, \cdot), \pi^t_h(\cdot \mid \x_h) - \pi^\star_h(\cdot \mid \x_h)\right\rangle \right] \nonumber
    \\&\le v + \E^{\pistar}\left[\sum_{h=1}^T\sum_{h=1}^H \tb_h^t(\x_h,\a_h)\right]  + \frac{1}{H}\cdot \sum_{t=1}^T\sum_{h=1}^H\E^{\pistar\circ_h \pi^t}\left[\tB_h^t(\x_h,\a_h)\right].
\label{eqn:regret condition}
\end{align}
Then, we have 
\begin{align*}
   \text{\rm Reg}_T \le v + 3\sum_{t=1}^T\sum_{h=1}^H\E^{\tp_h^t, \pi_h^t}\left[ \tb_{h}^t(\x_h,\a_h)\right].
\end{align*}
% \tp_h^t(\cdot|x,a)}\E_{\a_h \sim \pi_h^t(\cdot \mid \x_h)} \left[ b_{h}^t(\x_h,\a_h)\right].
%\cwcomment{The $\E^{\pistar\circ_h \pi^t}$ should be inside summation of $h$} \HL{Fixed}
\label{lem:dilated bonus}
\end{lemma}

In our case, for any $t \in [T]$, the bonuses $\Bhat_{1:H}^t$ defined in \cref{line:dilated} satisfy \cref{eqn:B condition} because for all $(x,a)\in \cX \times \cA$:
\begin{align*}
    \Bhat_h^t(x,a) &= b_h^t(x,a) + \left(1+\frac{1}{H}\right) \max_{P_h \in \cP_h^t} \E_{\x_{h+1}\sim P_h(\cdot \mid x,a)} \E_{\a_{h+1}\sim \pi^t_{h+1}(\cdot \mid \x_{h+1})}\left[\Bhat_{h+1}^t(\x_{h+1},\a_{h+1})\right],
    \\&= b_h^t(x,a) + \left(1+\frac{1}{H}\right) \E_{\x_{h+1}\sim \tp_h^t(\cdot \mid x,a)} \E_{\a_{h+1}\sim \pi^t_{h+1}(\cdot \mid \x_{h+1})}\left[\Bhat_{h+1}^t(\x_{h+1},\a_{h+1})\right]
    \\&\ge b_h^t(x,a) + \left(1+\frac{1}{H}\right)\cdot \E_{\x_{h+1}\sim P_h^\star(\cdot \mid x,a)} \E_{\a_{h+1}\sim \pi^t_{h+1}(\cdot \mid \x_{h+1})}\left[\Bhat_{h+1}^t(\x_{h+1},\a_{h+1})\right],
\end{align*}
where in the second step, we define
\begin{align*}
    \tp_h^t(\cdot|x,a) = \argmax_{P_h(\cdot|x,a):~P_h \in \cP_h^t} \left\{\E_{\x_{h+1}\sim P_h(\cdot \mid x,a)} \E_{\a_{h+1}\sim \pi^t_{h+1}(\cdot \mid \x_{h+1})}\left[\Bhat_{h+1}^t(\x_{h+1},\a_{h+1})\right]\right\},
\end{align*}
and the last step follows by \cref{lem:confidence set}.

To prove \eqref{eqn:regret condition} holds for our bonus, we use the following decomposition:
\begin{align}
    &\E^{\pistar}\left[\sum_{t=1}^T \sum_{h=1}^H\left\langle Q_{h}^{\pi^t}(\x_h,\cdot) - \Bhat_h^t(\x_h, \cdot), \pi_h^t(\cdot \mid \x_h) - \pi^\star_h(\cdot \mid \x_h)\right\rangle \right]\nn 
    \\&= \underbrace{\E^{\pistar}\left[\sum_{t=1}^T \sum_{h=1}^H\left\langle Q_{h}^{\pi^t}(\x_h,\cdot) - \Qhat_h^t(\x_h, \cdot), \pi_h^t(\cdot \mid \x_h) - \pi^\star_h(\cdot \mid \x_h)\right\rangle \right]}_{\textbf{Bias}}
  \nn  \\&\qquad + \underbrace{\E^{\pistar}\left[\sum_{t=1}^T \sum_{h=1}^H\left\langle \Qhat_{h}^t(\x_h,\cdot) - \Bhat_h^t(\x_h, \cdot), \pi_h^t(\cdot \mid \x_h) - \pi^\star_h(\cdot \mid \x_h)\right\rangle \right]}_{\textbf{FTRL}}, \label{eq:decompe}
\end{align}
where we recall that $\Qhat^t_h$ is defined as  
\begin{align}
\Qhat^t_h(x,a) \coloneqq Q^{\hatp^t,\pi^t}_h(x,a;\ell^t),  \nn
\end{align}
where $\widehat{P}^t$ is as in \cref{line:hatp}.
Moving define value function $\Vhat_h^{t}(x)  \coloneqq  \sum_{a \in \cA} \pi^t(a\mid x)\cdot \Qhat_h^t(x, a)$ and auxilary bonus
\begin{align*}
    B_h^t(x,a) = \frac{1}{2H}b_h^t(x,a) + \E^{\pi^t} \left[B_{h+1}^t(\x_{h+1}, \a_{h+1})\mid \x_h = x, \a_h =a\right].
\end{align*}
Note that $B_h^t(x,a) \le \frac{1}{2H}\cdot\Bhat_h^t(x,a)$ for all $x,a,h,t$ and we additioanly define $B_{H+1}^t(x,a) = 0$.

\paragraph{Bounding the bias term.} We now bound the bias term \eqref{eq:decompe}. We start by showing that $\left|\Qhat_{h}^t(x, a) - Q_{h}^{\pi^t}(x,a) \right|\le B_{h}^t(x,a)$ using induction. Assume $\left|\Qhat_{h+1}^t(x, a) - Q_{h+1}^{\pi^t}(x,a) \right|   \le B_{h+1}^t(x,a)$ for any $x \in \cX, a \in \cA$.  For any $x \in \cX, a \in \cA$, we have
\begin{align*}
    &\left|\Qhat_h^t(x, a) - Q_{h}^{\pi^t}(x,a) \right| 
    \\&=  \left|\E_{\x_{h+1} \sim \hatp^t_h(\cdot \mid x,a)}\left[\Vhat_{h+1}^{t}(\x_{h+1})\right] - \E_{\x_{h+1} \sim P_h^\star(\cdot \mid x,a)}\left[V_{h+1}^{\pi^t}(\x_{h+1})\right] \right|,
    \\&\le  \left|\E_{\x_{h+1} \sim \hatp^t_h(\cdot \mid x,a)}\left[\Vhat_{h+1}^{t}(\x_{h+1})\right] - \E_{\x_{h+1} \sim P_h^\star(\cdot \mid x,a)}\left[\Vhat_{h+1}^{t}(\x_{h+1})\right] \right| \nn \\
    & \quad +  \left|\E_{\x_{h+1} \sim P^\star_h(\cdot \mid x,a)}\left[\Vhat_{h+1}^{t}(\x_{h+1})\right]  - \E_{\x_{h+1} \sim P^\star_h(\cdot \mid x,a)}\left[V_{h+1}^{\pi^t}(\x_{h+1})\right] \right|,
    \\&\le H\left\|\hatp_{h}^t(\cdot\mid x,a) - P_h^\star(\cdot\mid x, a) \right\|_1 \nn \\ & \quad+  \E^{\pi^t} \left[\left|\Qhat_{h+1}^t(\x_{h+1}, \a_{h+1}) - Q_{h+1}^{\pi^t}(\x_{h+1},\a_{h+1})\right| \mid \x_h =x,\a_h=a \right],
    \\&\le H\left\|\hatp_{h}^t(\cdot\mid x,a) - P_h^\star(\cdot\mid x, a) \right\|_1 +  \E^{\pi^t} \left[B_{h+1}^t(\x_{h+1}, \a_{h+1})\mid \x_h=x,\a_h=a\right],
    \\&\le B_{h}^t(x,a),
\end{align*}
where the last step follows by definition of $b_h^t$ in \cref{line:bonus} of \cref{alg:full-info}. Since $Q_{H+1}^{\pi^t}(x,a) = \Qhat_{H+1}^t(x, a) = B_{H+1}^t(x,a) = 0$, by induction, we have for any $x \in \cX$, $a \in \cA$, $\left|Q_{h}^{\pi^t}(x,a) - \Qhat_h^t(x, a) \right| \le B_{h}^t(x,a)$. Using this, we bound the bias term in \eqref{eq:decompe} as follows:
\begin{align*}
    \textbf{Bias} &= \E^{\pistar}\left[\sum_{t=1}^T\sum_{h=1}^H \sum_{a \in \cA} \left(\pi_h^t(a\mid \x_h) - \pi^\star_h(a\mid \x_h)\right)  \left(Q_{h}^{\pi^t}(\x_h,a) - \Qhat_h^t(\x_h, a) \right)\right]
    \\&\le \sum_{t=1}^T\sum_{h=1}^H \E^{\pistar\circ_h \pi^t}\left[B_h^t(\x_h,\a_h)\right] +  \sum_{t=1}^T \sum_{h=1}^H\E^{\pistar}\left[B_h^t(\x_h,\a_h)\right],
    \intertext{and so, since $B_h^t(x,a) \le \frac{1}{2H}\Bhat_h^t(x,a)$   }
    &\le \frac{1}{2H}\cdot \sum_{t=1}^T \sum_{h=1}^H \E^{\pistar\circ_h \pi^t}\left[\Bhat_h^t(\x_h,\a_h) \right] + \frac{1}{2H}\cdot \sum_{t=1}^T\sum_{h=1}^H \E^{\pistar}\left[ b_h^t(\x_h,\a_h) \right] 
    \\&\qquad + \frac{1}{2H} \cdot \sum_{t=1}^T \sum_{h=1}^H \E^{\pistar\circ_{h+1}\pi^t} \left[\Bhat_{h+1}^t(\x_{h+1}, \a_{h+1})\right],\nn 
    \\&\le\frac{1}{H}\cdot  \sum_{t=1}^T \sum_{h=1}^H \E^{\pistar\circ_h \pi^t}\left[\Bhat_h^t(\x_h,\a_h)  \right] + \E^{\pistar}\left[\sum_{t=1}^T\sum_{h=1}^H b_h^t(\x_h,\a_h)\right].
\end{align*}
%\zm{justify the last inequality}
\paragraph{Bounding the FTRL term.} We now bound the FTRL term in \eqref{eq:decompe}.
For any $t \in [T]$, $h \in [H]$, $x \in \cX$ and $a\in \cA$, we have $|\Qhat_h^t(x,a)| \le H$,  $b_h^t(x,a) \le 4H^2$ and $\Bhat_h^t(x,a) \le 12H^3$ given $(1+\frac{1}{H})^H < e < 3$. Since $\eta = \frac{1}{13H^3\sqrt{T}}$, from \cref{lem:EXP bound}, we have
\begin{align*}
    \textbf{FTRL} &\le \frac{H \log|\cA|}{\eta} + \eta \sum_{h=1}^H \sum_{t=1}^T  \E^{\pistar \circ_h \pi^t} \left[\left(\Qhat_{h}^t(\x_h,\a_h) - \Bhat_h^t(\x_h, \a_h)\right)^2 \right],\nn 
    \\&\le \frac{H\log|\cA|}{\eta} + 2H^3\eta T + 288H^7\eta T,
    \\&= \order\left(H^4\sqrt{T}\log|\cA|\right).
\end{align*}
Thus, the bonuses $\Bhat_{1:H}^t$ in \cref{alg:full-info} also satisfy \cref{eqn:regret condition} with $v = \order\left(H^4\sqrt{T}\log|\cA|\right)$. Applying \cref{lem:dilated bonus}, we have
\begin{align} 
   &\text{\rm Reg}_T \nonumber
   \\&\le  \order\left(H^4\sqrt{T}\log|\cA|\right) + 3\sum_{t=1}^T \sum_{h=1}^H\E^{\tp_h^t, \pi_h^t}\left[ b_{h}^t(\x_h,\a_h)\right] \nonumber
   \\&\le \order\left(H^4\sqrt{T}\log|\cA|\right) + 3\sum_{t=1}^T\sum_{h=1}^H\E^{\pi^t}\left[b_{h}^t(\x_h,\a_h)\right] + 3\left(\sum_{t=1}^T \sum_{h=1}^H\E^{\tp_h^t, \pi_h^t}\left[ b_{h}^t(\x_h,\a_h)\right] -   \sum_{t=1}^T\sum_{h=1}^H\E^{\pi^t}\left[b_{h}^t(\x_h,\a_h)\right] \right) \nonumber
   \\&\le \order\left(H^4\sqrt{T}\log|\cA|\right) + 3\sum_{t=1}^T\sum_{h=1}^H\E^{\pi^t}\left[b_{h}^t(\x_h,\a_h)\right] +  3H^2\sum_{t=1}^T\sum_{h=1}^H\E_{(x, a) \sim d_h^{\pi^t}} \left[\left\|\tp_h\left(\cdot~|~x,a\right) - P_h^\star\left(\cdot~|~x,a\right)\right\|_1\right] \tag{\cref{lem:simulation}}
   \\&\le \order\left(H^4\sqrt{T}\log|\cA|\right) + 6\sum_{t=1}^T\sum_{h=1}^H\E^{\pi^t}\left[b_{h}^t(\x_h,\a_h)\right] \label{eqn:initial regret}
\end{align}

From \cref{lem:confidence set} and the triangle inequality, we have for any $P_h, P'_h \in  \cP_h^t$, we have
\begin{align*}
    &\sum_{i=1}^{t-1} \E^{\pi^i}\left[\left\|P_h(\cdot\mid \x_h, \a_h) - P'_h(\cdot\mid \x_h, \a_h)\right\|_1^2\right] \le 4c\log\left(|\Phi||\Upsilon| T\right).
\end{align*}
From \cref{lem:change of measure} and \cref{lem:cov bound}, for any $P_h, P_h' \in  \cP_h^t$, we have
\begin{align*}
    \sum_{t=1}^{T} \E^{\pi^t}\left[\left\|P_h(\cdot\mid \x_h, \a_h) - P_h'(\cdot\mid \x_h, \a_h)\right\|_1\right] \le \order\left(\sqrt{d |\cA| T \log(T)\log\left(|\Phi||\Upsilon| T\right)}\right) + 4d|\cA|.
\end{align*}
This implies 
\begin{align*}
    \sum_{t=1}^T\sum_{h=1}^H \E^{\pi^t}\left[b_{h}^t(\x_h,\a_h)\right] &= 2H^2\sum_{t=1}^T\sum_{h=1}^H\E^{\pi^t}\left[\max_{P_h, P_h' \in \cP_h^t} \|P_h(\cdot\mid \x_h, \a_h) - P_h'(\cdot\mid \x_h, \a_h)\|_1\right],
    \\&\le \order\left(H^3\sqrt{d |\cA| T \log(T)\log\left(|\Phi||\Upsilon|T\right)}\right) + 4dH^3|\cA|.
\end{align*}
Putting this back to \cref{eqn:initial regret}, we have
\begin{align*}
     \text{\rm Reg} \le  \order\left(H^4\sqrt{d|\cA|T}\log\left(|\cA| + |\Phi||\Upsilon| T\right) + dH^3|\cA|\right).
\end{align*}
