# Supplementary material for: Beating Adversarial Low-Rank MDPs with Unknown Transition and Bandit Feedback
Source: arXiv:2411.06739 source file (2024-11-11)
Supplement: Supplementary file 7 [file appendix_proof_oracleeff_ob.tex]

\section{Proof of \cref{thm:oraclealg} (Model-Free, Banfit Feedback)}
\label{sec:oracleeff}

\input{../analysis_performance_diff.tex}

\subsection{Bounding the Regret Term}
\input{../analysis_regret.tex}

\subsection{Bounding the Bias Term}
\input{../analysis_bound_bias.tex}

\subsection{Bounding the Regression Error}
\input{../analysis_regression_error.tex}

\subsection{Putting It All Together}
\input{../analysis_putting_all.tex}
